# Supplementary material for: Seeing to Generalize: How Visual Data Corrects Binding Shortcuts
Source: arXiv:2602.15183 source file (2026-02-16)
Supplement: Supplementary file 1 [file sec6_knockout.tex]

\section{Attention Knockout Analysis}
\label{app:knockout}

We present the aggregate attention knockout results in Figure~\ref{fig:knockout_all}. These heatmaps show the average impact on task performance when individual attention heads are masked, averaged across all seeds for the respective model types.

\begin{figure*}[h]
    \centering
    \begin{subfigure}[b]{0.48\textwidth}
        \centering
        \includegraphics[width=\linewidth]{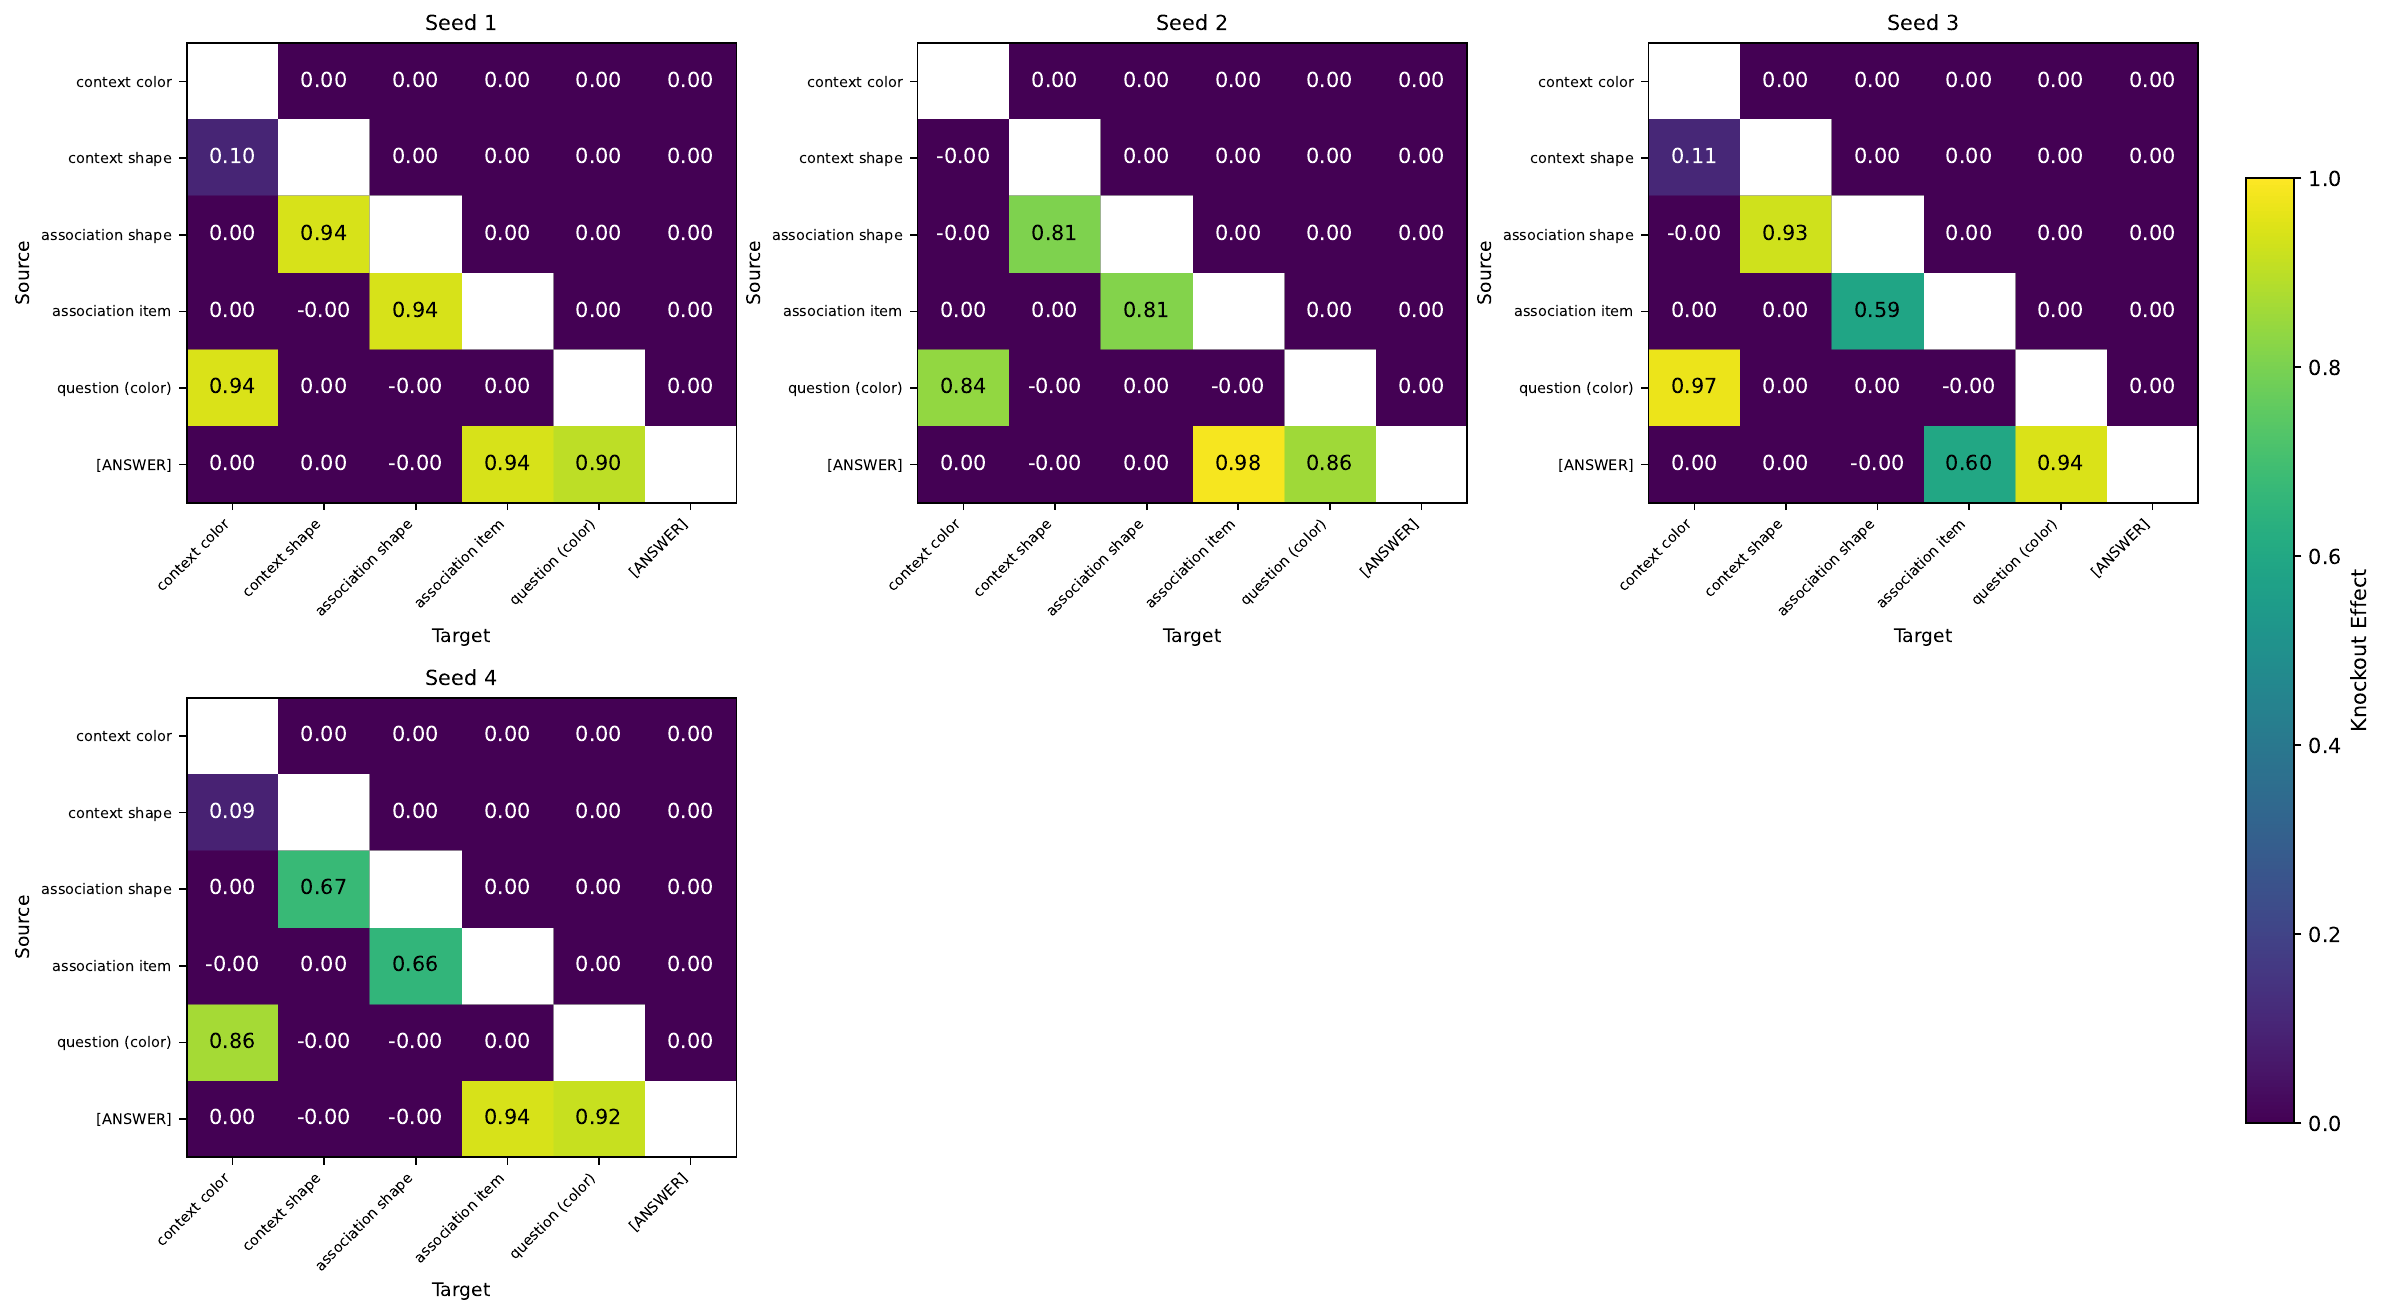}
        \caption{Text-Only ($\mathcal{M}_{\text{text}}$) - All Seeds}
        \label{fig:knockout_text_all}
    \end{subfigure}
    \hfill
    \begin{subfigure}[b]{0.48\textwidth}
        \centering
        \includegraphics[width=\linewidth]{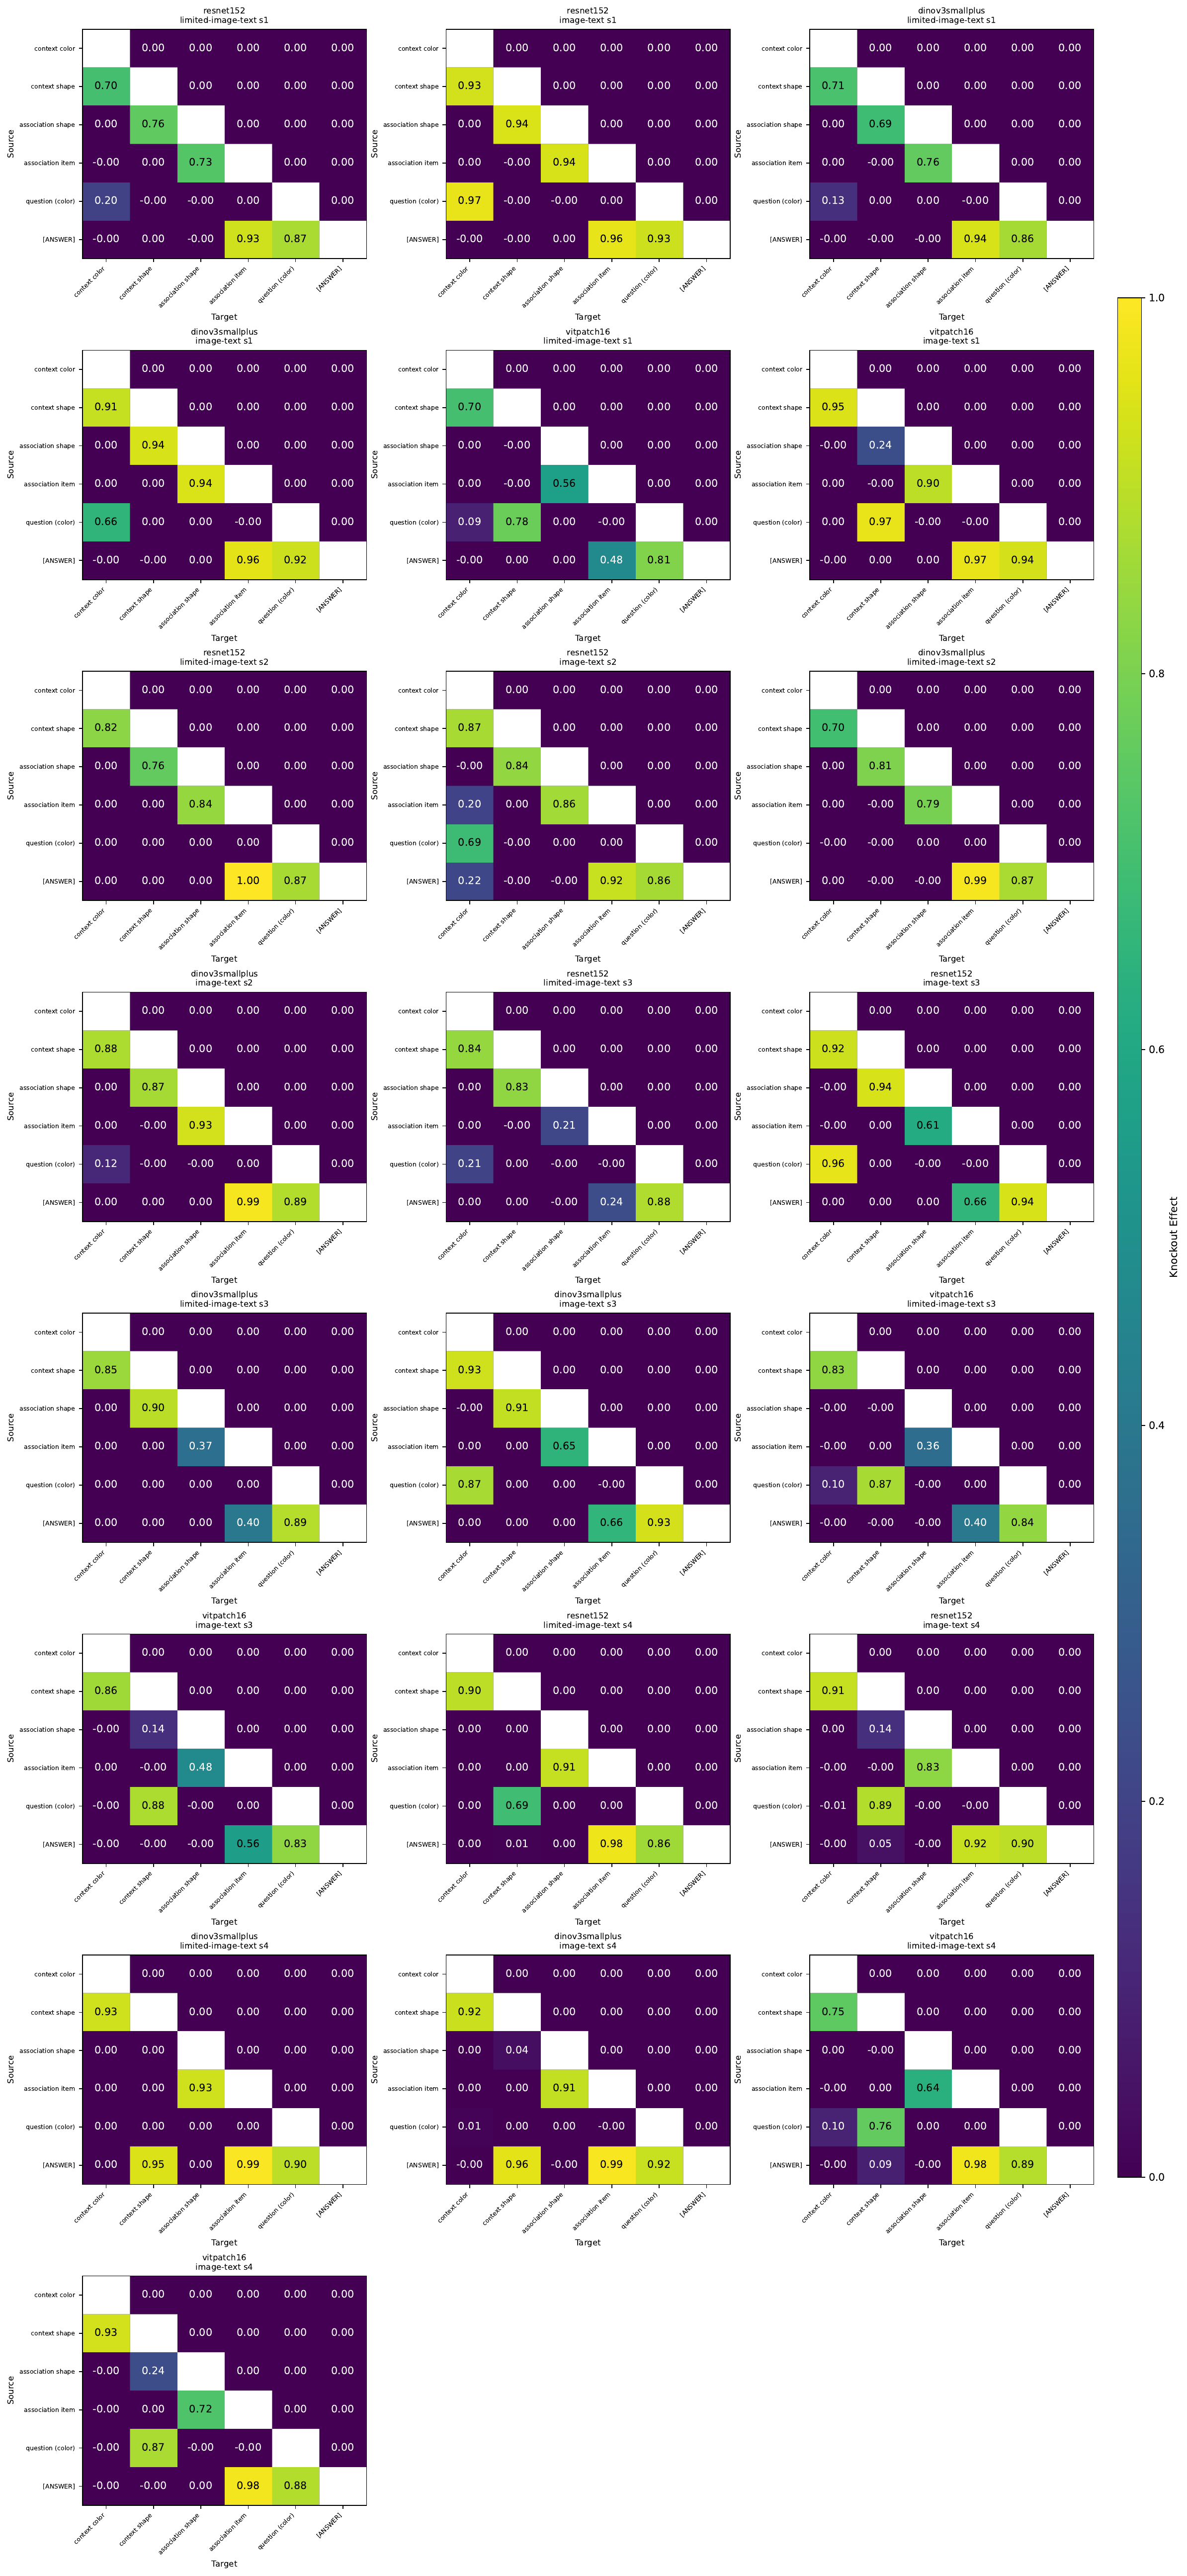}
        \caption{Image-Text ($\mathcal{M}_{\text{image-text}}$) - All Runs}
        \label{fig:knockout_image_text_all}
    \end{subfigure}
    \caption{\textbf{Aggregate Attention Knockout Analysis.} Average impact of head masking across all experimental runs. The positional text models consistently rely on a single critical circuit, while the lexical image-text models utilize more distributed mechanisms.}
    \label{fig:knockout_all}
\end{figure*}
