# Supplementary material for: Seeing to Generalize: How Visual Data Corrects Binding Shortcuts
Source: arXiv:2602.15183 source file (2026-02-16)
Supplement: Supplementary file 2 [file sec6_linear_probe.tex]

\section{Linear Probe Analysis}
\label{app:linear-probe}

In this section, we provide the aggregate linear probe results across all runs. Figure~\ref{fig:linear_probes_all} illustrates the average probing accuracy for task-relevant features, confirming that the trends observed in the representative examples (Figure~\ref{fig:linear_probes}) are consistent across random seeds and different image encoders.

\begin{figure*}[h]
    \centering
    \begin{subfigure}[b]{0.48\textwidth}
        \centering
        \includegraphics[width=\linewidth]{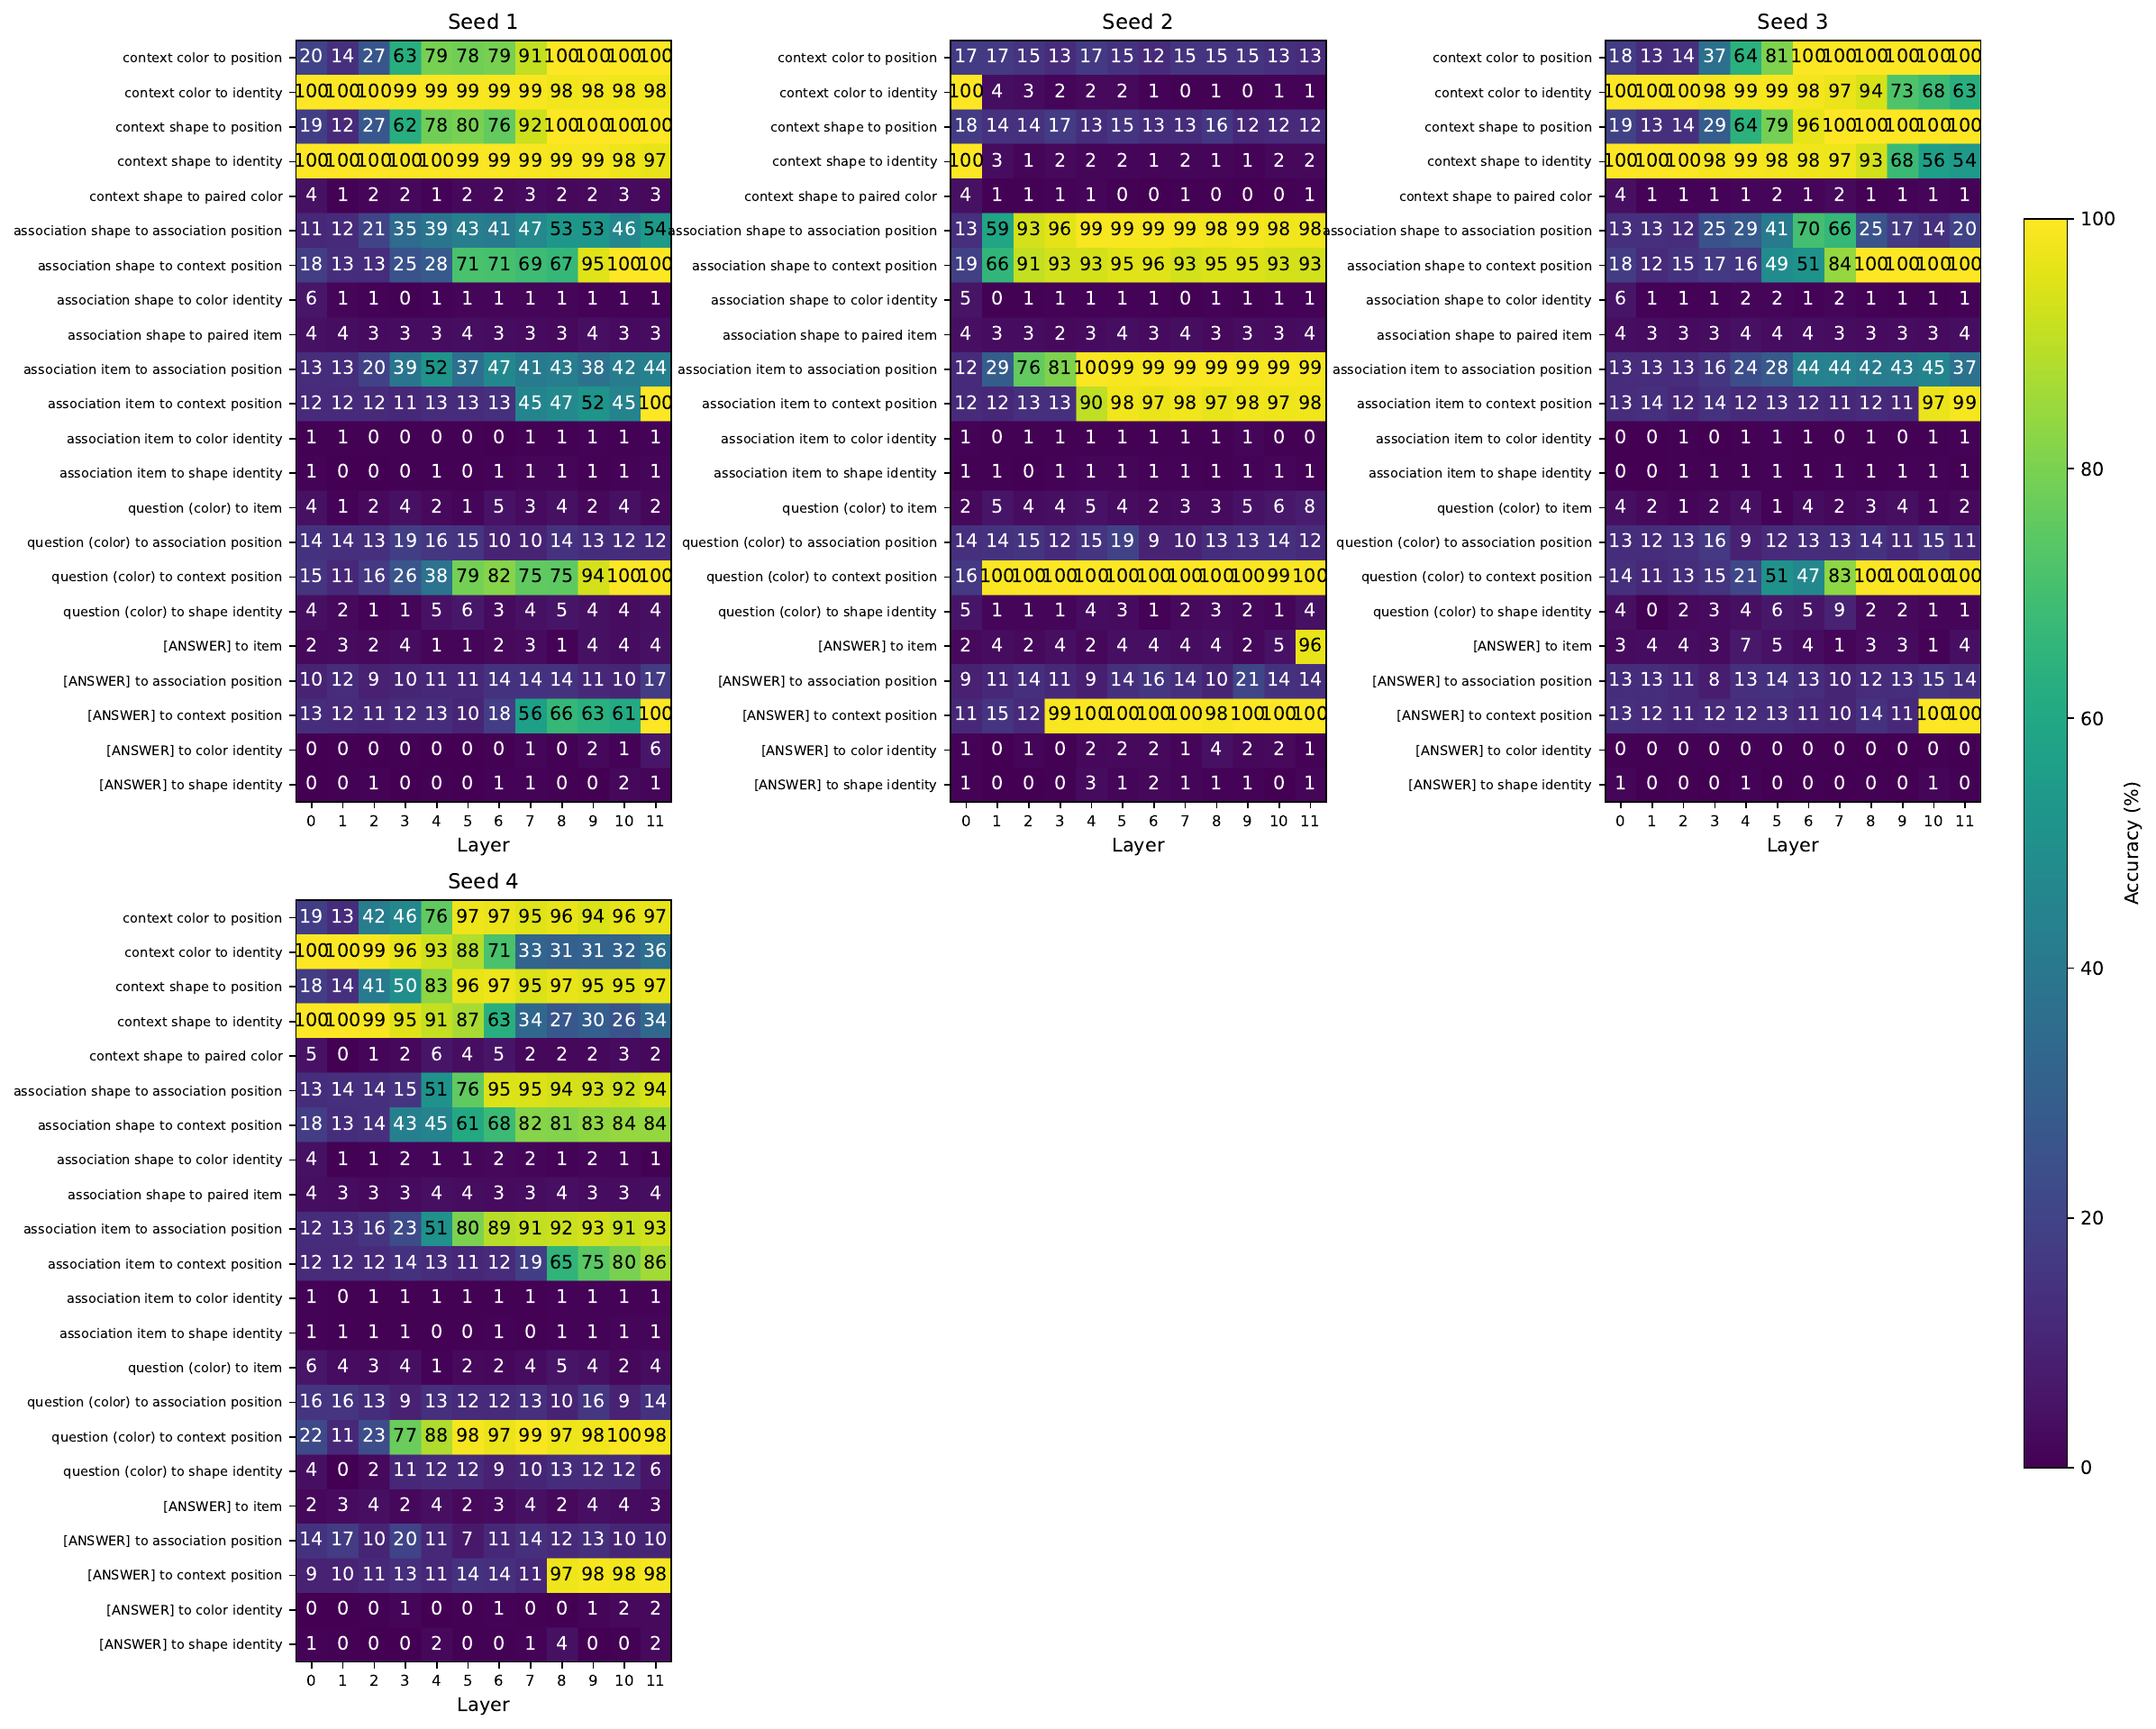}
        \caption{Text-Only ($\mathcal{M}_{\text{text}}$) - All Seeds}
        \label{fig:probe_text_all}
    \end{subfigure}
    \hfill
    \begin{subfigure}[b]{0.48\textwidth}
        \centering
        \includegraphics[width=\linewidth]{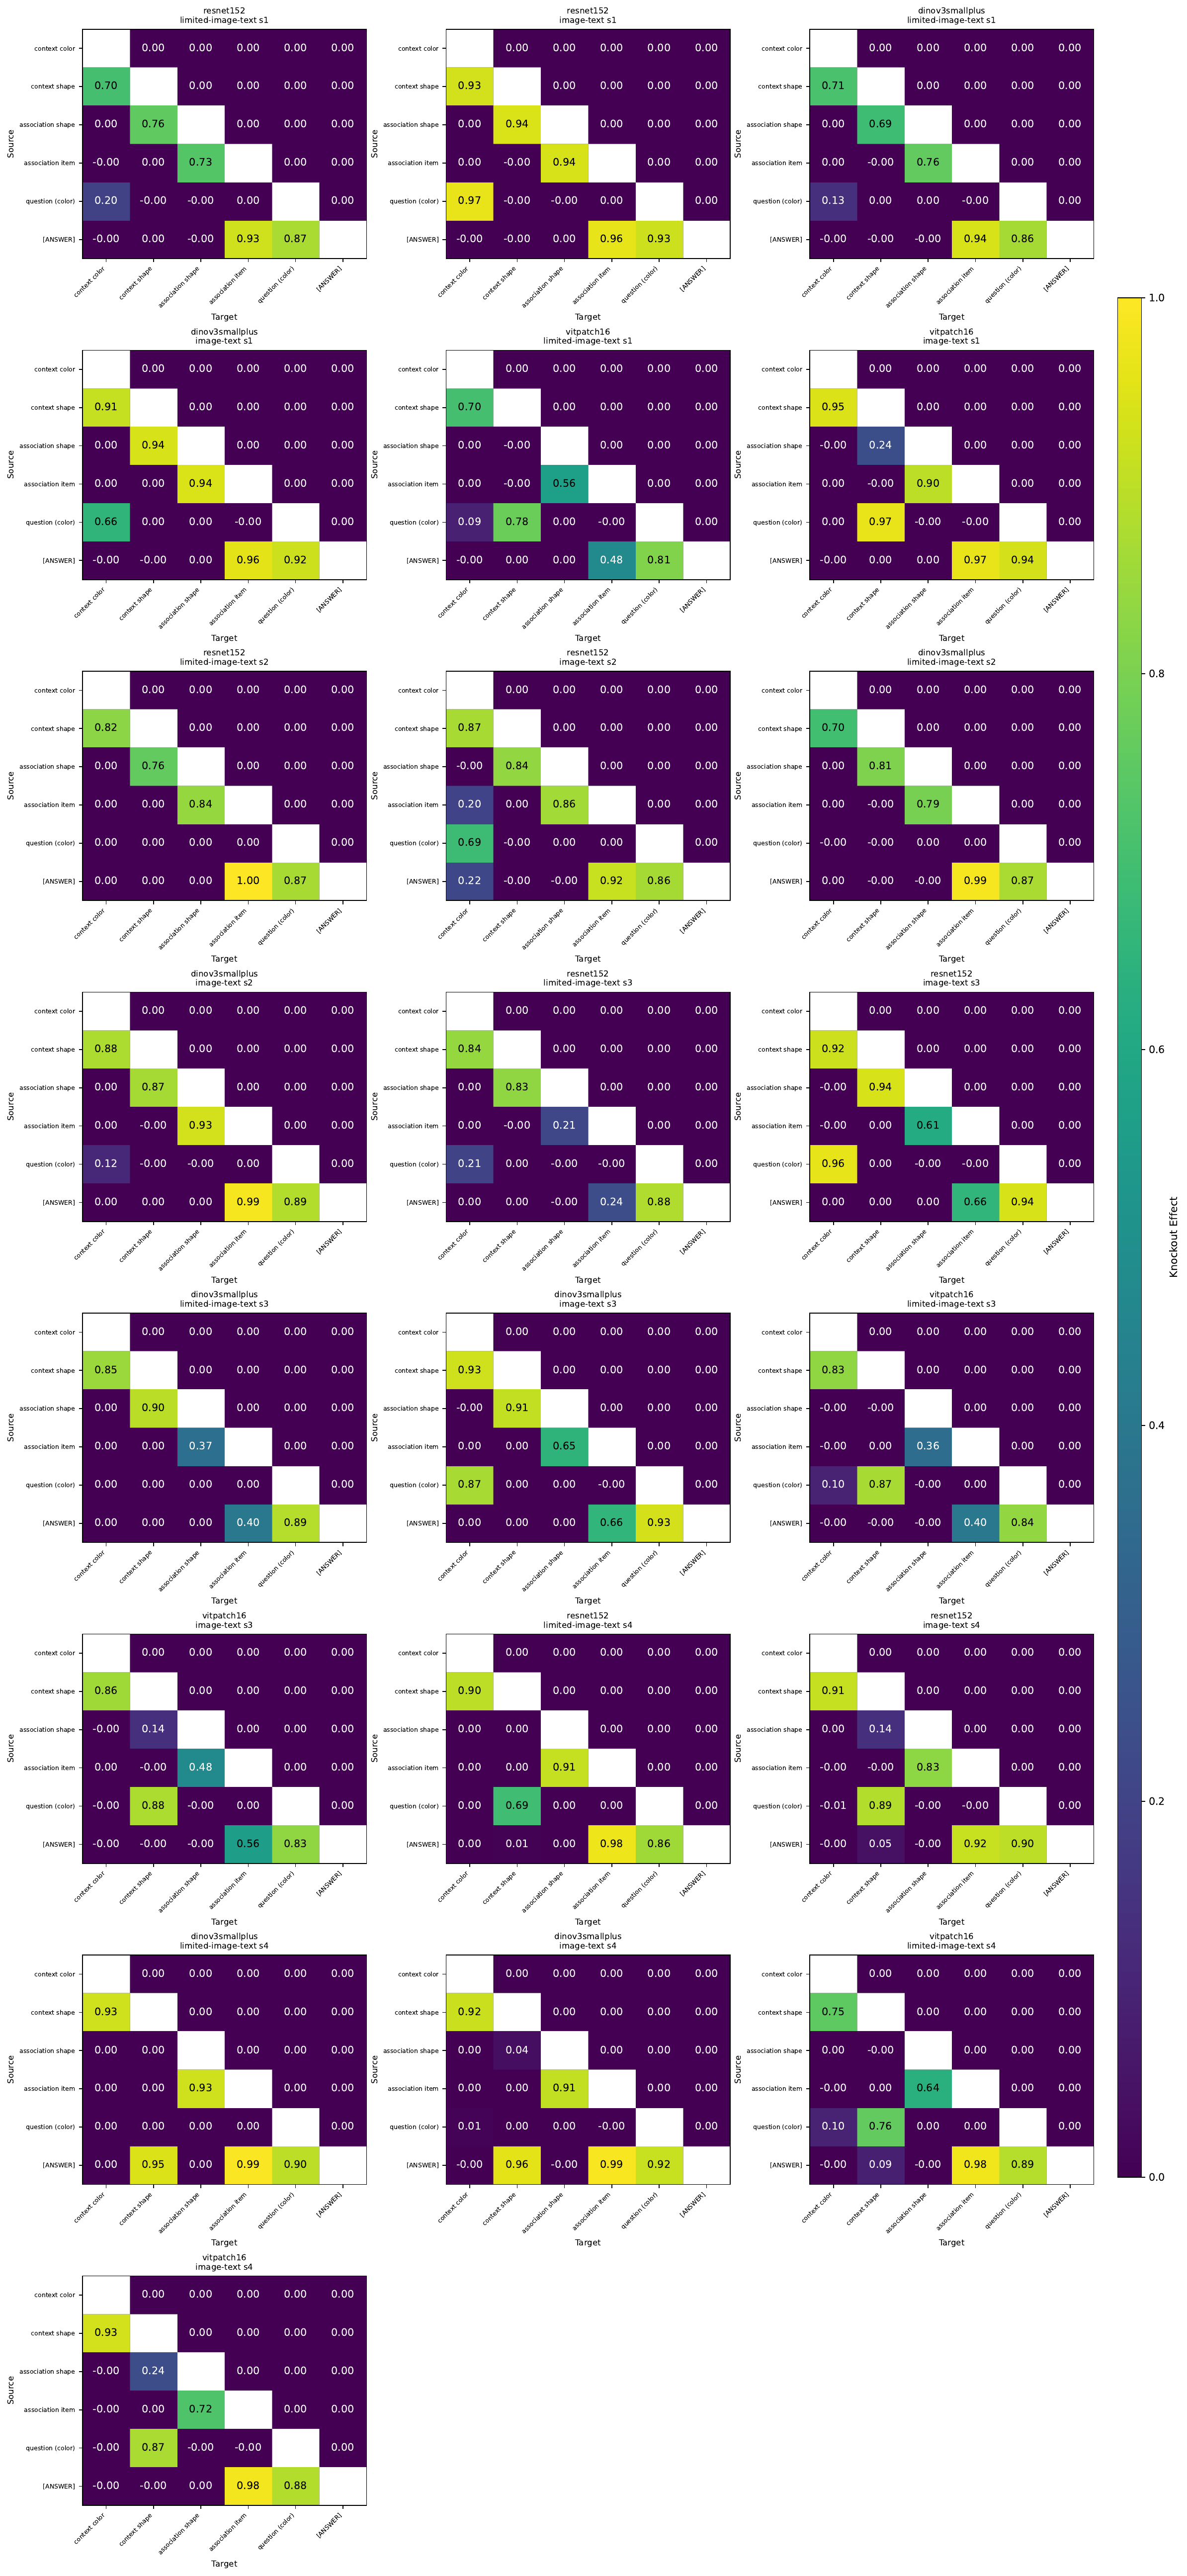}
        \caption{Image-Text ($\mathcal{M}_{\text{image-text}}$) - All Runs}
        \label{fig:probe_image_text_all}
    \end{subfigure}
    \caption{\textbf{Aggregate Linear Probe Analysis.} Average probing accuracy across all experimental runs.}
    \label{fig:linear_probes_all}
\end{figure*}
